# Supplementary material for: Soft Rasterizer: A Differentiable Renderer for Image-based 3D Reasoning
Source: arXiv:1904.01786 source file (2019-04-03)
Supplement: Supplementary file 4 [file suppl_video.tex]

\section{Video}
\label{sec:suppl_video}

We also include a \textit{supplemental video} that provides animated visualization of our results. 
Please refer to the video for more details. 

%In the \textit{supplemental video}, we show the animated visualization of (1) our forward rendering; (2) more reconstruction results; (3) the mesh deformation procedure and (4) the fitting process of SMPL pose optimization.
